# Supplementary material for: Multi-transversals for Triangles and the Tuza's Conjecture
Source: arXiv:2001.00257 source file (2021-02-03)
Supplement: Supplementary file 2 [file appendix.tex]

\appendix

\section{Omitted Claims from Section~\ref{sec:overview}}

\subsection{Proof of Proposition~\ref{prop:structures-solution}}

\begin{claim}
\label{clm:common-anchoring}
For any solution triangle $\psi$, if there are two triangles singly-attached to $\psi$, then these two attached triangles either have the same base, or the same anchoring vertex.
%For any solution triangle, there cannot exist two attached triangles with different base edges and different anchoring vertices.
\end{claim}
\begin{proof}
Otherwise if $\psi$ is the solution triangle and $t', t''$ are the singly-attached triangles of $\psi$ with different base edges and different anchoring vertices, then $\Nu \cup \{t', t''\} \setminus \{\psi\}$ is a better solution, contradicting the optimality of $\Nu$.
\end{proof}

\begin{corollary}
\label{cor:type-2}
There is no type-$2$ solution triangle.
\end{corollary}
\begin{proof}
% By claim~\ref{clm:common-anchoring}, there exists only one anchoring vertex.
% vertices of any type-$2$ green triangle plus the corresponding anchoring vertex form $K_4$, and this triangle is actually type-$3$.
% \pattara{Is this better than the previous proof?}
By claim~\ref{clm:common-anchoring}, for any solution type-$2$ triangle $\psi$, the two singly-attached triangles attached to different edges of $\psi$ must share their anchoring vertex and there cannot be any other singly-attached triangle attached to $\psi$. This implies that the vertices of $\psi$ plus the anchoring vertex induce a $K_4$, hence in fact it is a type-$3$ triangle.
\end{proof}

\begin{corollary}
\label{cor:type-3}
For any type-$3$ triangle in $\tset$, there are exactly three attached triangles and one anchoring vertex.
% All type-$3$ triangles in $G$ supports exactly three attached triangles with a common landing vertex.
\end{corollary}
\begin{proof}
Follows directly by claim~\ref{clm:common-anchoring}.
\end{proof}

\subsection{Proof of Proposition~\ref{prop:structures-doubly-attached}}
%\sumi{Fixed some cases in the statement of this proposition.}
\label{proof-prop:doubly-attached}

First we argue that there is no $t: type(t) = [3,3]$.
Assume there is doubly-attached triangle $t \in \tset$ attached to two solution triangles of type-$3$, $\psi_1$ and $\psi_2$.
Note that:
\begin{itemize}
    \item The anchoring vertices (possibly same) of $\psi_1$ and $\psi_2$ cannot be in $V(\psi_1) \cup V(\psi_2)$; otherwise, some of the attachments would have been doubly-attached, rather than singly-attached.
    \item Let $e_1$ and $e_2$ be edges in $E(\psi_1)$ and $E(\psi_2)$ not using $V(\psi_1) \cap V(\psi_2)$. Notice that these two edges are vertex-disjoint.
\end{itemize}

There exists two edge-disjoint singly-attached triangles $t_1 \ni e_1$ and $t_2 \ni e_2$ attached to $\psi_1$ and $\psi_2$ respectively. $t_1$ and $t_2$ are edge-disjoint because $e_1$ and $e_2$ are vertex-disjoint.
Hence, $\Nu \cup \{t_1, t_2, t\} \setminus \{\psi_1, \psi_2\}$ is a larger set of edge disjoint triangles, which contradicts the optimality of $\Nu$ (see Fig.~\ref{fig:blue-2-swap-2-type-3} for illustration).

\input{tikz_figures/blue-2-swap-2-type-3}

% O.w. there exists a $2$-swap.

Now consider a doubly-attached triangle $t$ where $type(t) = [1,3]$.
Let $\psi_1$ and $\psi_2$ be solution triangles which $t$ is doubly-attached to.
WLOG, let $\psi_1$ be type-$1$.
If  $base(\psi_1) \in E(t)$, then we are done.
For the rest of the proof, we assume that the base $e_1 \notin E(t)$.

First, if $|\CL_{sin}(\psi_1)| > 1$, then there is an anchoring vertex of $\psi_1$ is not in $V(t)$. Let $t_1$ be any singly-attached triangle using this anchor. Notice that $E(t_1)$ and $E(t)$ are disjoint.
Since $\psi_2$ is type-$3$, there is a singly-attached triangle $t_2$ whose base is vertex-disjoint from $\psi_1$.
Notice that $t,t_1, t_2$ are edge-disjoint triangles (an easy way to see this is that each pair of them has at most one vertex in common).
We could exchange the solution by removing $\{\psi_1, \psi_2\}$ and adding $\{t, t_1, t_2\}$.
Hence, it must be that $|\CL_{sin}(\psi_1)| = 1$ and that the anchoring vertex is in $V(t)$.

\subsection{Proof of Proposition~\ref{prop:type-[1-1]}}
\label{proof-prop:type-[1-1]}
Notice that $t$ is a type-$[1,1]$ triangle. Let $\psi_1$ and $\psi_2$ be solution triangles which $t$ is doubly-attached to.
If $E(t)$ contains $base(\psi_1)$ or $base(\psi_2)$, then we are done by Proposition~\ref{prop:type-[1-1]}.\ref{itm:base-edge}. Now we assume that $\{base(\psi_1), base(\psi_2)\} \cap E(t) = \varnothing$. 
If $|CL_{sin}(\psi_1)| \geq |CL_{sin}(\psi_2)| >1$, then there exists two singly-attached triangles $t_1, t_2$ attached to $base(\psi_1), base(\psi_2)$ respectively such that $anchor(t_1) \neq anchor(t_2)$ and edge-disjoint from $t$. In this case, we let $\Nu^\prime = (\Nu \setminus \{\psi_1, \psi_2\}) \cup \{t, t_1, t_2\}$. Since $\Nu^\prime$ has more triangle than $\Nu$, it contradicts optimality of $\Nu$. Now by renaming, let us assume $|CL_{sin}(\psi_1)| = 1$. Let $t_1$ be the singly-attached triangle of $\psi_1$. If $anchor(t_1) \in E(t)$ then we are done. If not, then if $|CL_{sin}(\psi_2)|>1$ we have an improving swap using the an argument similar to the previous case. If $|CL_{sin(\psi_2)}| = 1$, let $t_2$ be the singly-attached triangle. If $anchor(t_2) \in E(t)$ then we are done by renaming. Else if $base(\psi_1) \cap base(\psi_2) = \varnothing$ or $anchor(t_1) \neq anchor(t_1)$, then still $\Nu^\prime = (\Nu \setminus \{\psi_1, \psi_2\}) \cup \{t, t_1, t_2\}$ is an improving swap because $t_1, t_2, t$ are edge disjoint since they share at most one vertex with each other. Hence the only remaining possibility is that $anchor(t_1) = anchor(t_2)$ and $base(\psi_1) \cap base(\psi_2) \neq \varnothing$, which is our Proposition~\ref{prop:type-[1-1]}.~\ref{itm:pair}. Hence, we conclude the proof.

% \end{itemize}

\subsection{Proof of Proposition~\ref{prop:structures-hollow}}
%\sumi{Fixed some cases in the statement of this proposition.}
\label{proof-prop:hollow}

First we argue that there is no $t: type(t) = [3,3, 3]$.
Assume there is a hollow triangle $t \in \tset$ attached to three solution triangles of type-$3$, $\psi_1$, $\psi_2$ and $\psi_3$.
Notice that $|\bigcup_{i=1}^{3} V(\psi_i)| = 6$ since these solution triangles cannot share edges. For any $i$, let $v_i = V(\psi) \setminus V(t)$ be an only vertex of $\psi_i$ that is not in $V(t)$. Let $cv_{ij} \in V(\psi_i) \cap V(\psi_j)$ be the vertex shared between $\psi_i$ and $\psi_j$. It is possible that all $a_i = anchor(\psi_i)$ are the same vertex for all $i$. Consider the set $S$ of four disjoint triangles $\{\Delta_{v_1 cv_{12} a_1} , \Delta_{v_2 cv_{23} a_2}, \Delta_{v_3 cv_{13} a_3}, t \}$.
Since $ \Nu^\prime =  (\Nu \setminus \bigcup_{i=1}^{3} \psi_i) \cup S$ is a set of disjoint triangle of size $|\Nu| + 1$, then it contradicts the fact that $\Nu$ is optimal.

Now we consider the case where $type(\psi_1) =1$. There are three sub cases.

The first sub case is when $type(t) = [1, 3, 3]$. Assume that $base(\psi_1)$ is not in $t$. In this case, $anchor(\psi_2) \neq anchor(\psi_3)$ or the base edge of $\psi_1$ will be in $t$. 
WLOG, assume that the $base(\psi_1)$ is $\overbar{v_1 cv_{12}}$. 

We then can select the set $S$ of four disjoint triangles $\{\Delta_{v_2 cv_{23} a_2}, \Delta_{v_3 cv_{23} a_3}, t_1 \in \CL_{sin}(\psi_1), t\}$.
Since $\Nu^\prime =  (\Nu \setminus \bigcup_{i=1}^{3} \psi_i) \cup S$ is a set of disjoint triangle of size $|\Nu| + 1$, then it again is a contradiction.

The second sub case is when $type(t) = [1, 1, 3]$. 
Assume that $\{base(\psi_1), base(\psi_2)\} \cap E(t) = \varnothing$.
Let $t_1 \in \CL_{sin}(\psi_1)$ and $t_2 \in \CL_{sin}(\psi_2)$ be two disjoint singly-attached triangles. There exists such triangles or $\psi_1$ and $\psi_2$ will share a single anchoring vertex. Let $t_3$ be a singly-attached triangle of $\psi_3$, which is disjoint from $t_1$ and $t_2$. There exists such $t_3$ or $t_1$ and $t_2$ would share their anchoring vertex.
Let $S= \{t_1, t_2, t_3, t\}$ be a set of four disjoint triangles. 
Since $ \Nu^\prime =  (\Nu \setminus \bigcup_{i=1}^{3} \psi_i) \cup S$ is a set of disjoint triangle of size $|\Nu| + 1$, then it again is a contradiction.

Now come the third sub case when $type(t) = [1, 1, 1]$.
Assume that $\{base(\psi_1), base(\psi_2), base(\psi_3)\} \cap E(t) = \varnothing$. If these three base edges share no vertex, then it is easy to see that there exists three disjoint singly-attached triangles $t_1, t_2, \text{ and } t_3$, attaching to $\psi_1, \psi_2, \text{ and } \psi_3$ in respective order.
Let $S= \{t_1, t_2, t_3, t\}$ be a set of four disjoint triangles. 
Since $ \Nu^\prime =  (\Nu \setminus \bigcup_{i=1}^{3} \psi_i) \cup S$ is a set of disjoint triangle of size $|\Nu| + 1$, then it again is a contradiction.

Otherwise, WLOG, assume that $base(\psi_1)$ and $base(\psi_2)$ share the vertex $cv(\psi_1, \psi_2)$. We are still able to select two disjoint singly-attached triangle $t_1 \in \CL_{sin}(\psi_1)$ and $t_2 \in \CL_{sin}(\psi_2)$ as they are not sharing a single anchoring vertex.
Let $S= \{t_1, t_2, t_3 \in \CL_{sin}(\psi_3), t\}$ be a set of four disjoint triangles. 
Since $ \Nu^\prime =  (\Nu \setminus \bigcup_{i=1}^{3} \psi_i) \cup S$ is a set of disjoint triangle of size $|\Nu| + 1$, then it again is a contradiction.

This conclude the proof.

\section{Omitted Claims from Section~\ref{sec:order-2}}

Let us first define some notations that will be used throughout the proof.
First, for any triangle $t$, as in other sections, we let $V(t)$ be set of vertices of this triangle.
Also, for set of triangles $T$, we let $V(T)$ be set of vertices of these triangles.
We might abuse notation and use $t$ as $\{t\}$. For example, for two triangles
 $t_1$ and $t_2$, $V(t_1 \cup t_2) = V(t_1) \cup V(t_2)$ is the set of vertices of these two triangles.

\subsection{Proof of Lemma~\ref{lem:demanding-lemma}}

\begin{proof}
   First, as mentioned in the distribution scheme, there are five local structures that we can see when a triangle has a demanding edge. Let $\psi$ be the type-$0$ triangle. Let $t$ be the triangle next to $\psi$ where the demand is needed. Then $t$ is either
   \begin{enumerate}
      \item \cat{type-$[0,3]$ doubly-attached triangle} See fig~\ref{fig:blue-0,3-demanding}.
      \item \cat{type-$[0,1]$ doubly-attached triangle} In this case, the edge shared with the type-$1$ triangle must be drained edge.
      See fig~\ref{fig:blue-0,1-demanding}.
      \item \cat{type-$[0,3,3]$ hollow triangle} See fig~\ref{fig:hollow-0,3,3-demanding}.
      \item \cat{type-$[0,1,3]$ hollow triangle} As in the previous case, the edge shared with the type-$1$ triangle must be poor edge. See fig~\ref{fig:hollow-0,1,3-demanding}.
      \item \cat{type-$[0,1,1]$ hollow triangle} the two other solution edges of $t$ are poor edges. See fig~\ref{fig:hollow-0,1,1-demanding}. Note that the type-$3$ triangles which we see in the figure cannot be merged into one triangle as $\psi$ will no longer be type-$0$.
    \end{enumerate}

    \begin{claim}
    \label{clm:disjoint-type3}
      For any of the above cases, all the type-$3$ triangles involved in either the doubly attached or hollow triangle directly or making base edge of some type-$1$ poor are disjoint.
   \end{claim}
   \begin{proof}
      Either it is not possible to draw the case with common type-$3$ triangle or it violates the fact that 
     $|\CL_{sin}(\psi)| = 0$.
    %   the type-$0$ triangle does not support any triangle.
      \input{tikz_figures/hollow-0-1-1-with-itself}
   \end{proof}

    We will show that it is impossible to have a type-$0$ triangle with two demanding edges. For contradiction suppose the lemma is not true, then we have a type-$0$ triangle $\psi$ with two demanding edges $e_{\ell}$ and $e_r$. Think of $e_{\ell}$ as the {\em left} demanding edge and $e_r$ as the {\em right} demanding edge. We will follow this naming convention in the proof and the figures to help visualize various cases. 
    
    On each side, we will see one of five cases above.

    One might categorize these structures by the types of triangles adjacent to $\psi$, which are combinations of doubly-attached and hollow triangles. We name these two triangles $t_\ell$ and $t_r$. Remember that both $t_\ell$ and $t_r$ demand credit from $\psi$ (so that $\psi$ has two demanding edges).

    \begin{lemma}
      \label{lem:both-doubly-attached-demanding}
      If $t_\ell$ is a doubly-attached triangle, then $t_r$ cannot be a doubly-attached triangle.
    \end{lemma}

    \begin{proof}
      Suppose not, then $t_\ell$ and $t_r$ are doubly-attached triangles sharing demanding edges $e_\ell \neq e_r$ with $\psi$. Let $\psi_\ell$ be the other solution triangle that shared an edge with $t_\ell$ and $\psi_r$ be the other solution triangle that shared an edge with $t_r$. Let $v_\ell$ be the common vertex of $\psi$ and $\psi_\ell$. Let $v_r$ be the common vertex of $\psi$ and $\psi_r$ (possibly $v_r = v_\ell$). Similarly, let $u_\ell$ to be the other vertex of $\psi$ in $t_\ell$ and $u_r$ to be the other vertex of $\psi$ in $t_r$ (possibly $u_r = u_\ell$). Note that either $v_r = v_\ell$ or $u_r = u_\ell$ but not both. 
      If $u_r = u_\ell$ and $v_r \neq v_\ell$, we call $u_r = u_\ell$ as $u$ else we call $v_r = v_\ell$ as $v$. Note that $e_\ell = \overbar{u_\ell v_\ell}$ and $e_r = \overbar{u_r v_r}$ in both the cases. Let $w_\ell$ be the second common vertex of $\psi_\ell$ and $t_\ell$ and; $w_r$ be the the second common vertex of $\psi_r$ and $t_r$. Finally, let $v_{\ell\ell}$ be the third vertex of $\psi_\ell$ and $v_{rr}$ be the third vertex of $\psi_r$ (see fig~\ref{fig:demand-two-doubly-attached-two-type-3}).
      Up to renaming $\psi_\ell$ and $\psi_r$, there are three cases.
      \begin{enumerate}
         \item \cat{$\psi_\ell$ and $\psi_r$ are type-$3$}
         There are several sub-cases here.
         
         In case when $u_r \neq u_\ell$ and $v$ is a common vertex of $\psi, \psi_\ell, \psi_r$, then it could be that $\psi_\ell = \psi_r$ (say $\psi^3$). Then $v_{rr} = w_\ell$ and $v_{\ell\ell} = w_r$ (see fig~\ref{fig:demand-two-doubly-attached-one-type-3-common}). But this is impossible because there is a solution improving $2$-swap by replacing the set of triangles $\sset=\{\psi, \psi^3\}$ by the bigger set $\sset'= \{t_\ell, t_r, t'\}$,
         where $t'$ is the singly-attached triangles of $\psi^3$  attached to edge $E(\psi) \setminus E(t_l \cup t_r)$.
         
         \input{tikz_figures/demand-two-doubly-attached-one-type-3-common}

         In the case when $u$ is a common vertex and $v_r \neq v_\ell$, it is impossible that $\psi_\ell = \psi_r$ because $\overbar{v_\ell v_r}$ is in $E(\psi)$. 
        
         Now both the cases when $\psi_\ell \neq \psi_r$ are impossible because there is a solution improving $3$-swap by replacing the set of triangles $\sset=\{\psi, \psi_\ell, \psi_r\}$ by the bigger set $\sset'= \{t'_\ell, t_\ell, t_r, t'_r\}$,
         where $t'_\ell$ and $t'_r$ are the singly-attached triangles of $\psi_\ell$ and $\psi_r$ attached to edge $\overbar{w_\ell v_{\ell\ell}}$ and $\overbar{w_r v_{rr}}$ respectively. It is easy to that the triangles in $\sset'$ are edge disjoint even in the worst case when $anchor(\psi_\ell) = anchor(\psi_r)$. For illustration see fig~\ref{fig:demand-two-doubly-attached-two-type-3}.

         \input{tikz_figures/demand-two-doubly-attached-two-type-3}

         \item \cat{$\psi_\ell$ is type-$3$ and $\psi_r$ is type-$1$}
         Since $\psi_r$ is type-$1$, the edge $e_r = \overbar{v_r w_r}$ shared between $t_r$ and $\psi_r$ must be a poor base edge. This also indicates that there exists a doubly-attached triangle $t_{rr}$ which share an edge with $\psi_r$, a type-$3$ triangle $\psi_{rr}$ and non-solution edge of the only singly attached-attached triangle of $\psi_r$. Note that, $v_{rr}$ will be the common vertex between $\psi_r$ and $\psi_{rr}$. Let $w_{rr}$ be the other vertex of $\psi_{rr}$ contained in $t_{rr}$ and $x_{rr}$ be the third vertex of $\psi_{rr}$ (see fig~\ref{fig:demand-two-doubly-attached-one-type-3-one-type-1}). If $\psi_\ell \neq \psi_{rr}$, then in both cases when $v_\ell=v_r=v$ or when $u_\ell=u_r=u$ are impossible since there exists a solution improving $4$-swap by replacing the set of triangles $\sset=\{\psi, \psi_\ell, \psi_r, \psi_{rr}\}$ by set $\sset'= \{t'_\ell, t_\ell, t_r, t_{rr}, t'_r\}$, where $t'_\ell$ and $t'_r$ are the singly-attached triangles of $\psi_\ell$ and $\psi_{rr}$ attached to edge $\overbar{w_\ell v_{\ell\ell}}$ and  $\overbar{w_{rr} x_{rr}}$ respectively. It is easy to that the triangles in $\sset'$ are edge disjoint even in the worst case when $anchor(\psi_\ell) = anchor(\psi_{rr})$. For illustration see fig~\ref{fig:demand-two-doubly-attached-one-type-3-one-type-1}).

         \input{tikz_figures/demand-two-doubly-attached-one-type-3-one-type-1}

         Otherwise, $\psi_\ell = \psi_{rr}$ (say $\psi^3$). 
         In this case, $v_\ell$ and $v_r$ cannot be the same since then for $\psi_r$ the $anchor(\psi_r)$ needs to be either $w_\ell$ or $v_{\ell\ell}$ and; the base edge needs to be $\overbar{v w_r}$, but the edges $\overbar{v w_\ell}$ and $\overbar{v v_{\ell\ell}}$ both are solution edges of $\psi_\ell$ hence cannot be non-solution edges for the singly-attached triangles of $\psi_r$.
         
         Now we need to deal with the case when $\psi_\ell = \psi_{rr} = \psi^3$ and $u_\ell=u_r=u$.
         In this case, $\psi^3$ share the vertex $v_\ell$ with $\psi$ to create $t_\ell$ and $v_{rr}$ vertex with $\psi_r$ since $e_r=\overbar{v_rw_r}$ is the poor base edge of $\psi_r$. Note that the third vertex of $\psi^3$ will be $w_\ell = w_{rr}$ (say $w$). Now there will be non-solution edge $uw$ to complete the doubly-attached $t_\ell$ and; edges $v_rw$ and $w_rw$ to complete the singly attached triangle of $\psi_r$. But it is impossible since $\psi$ cannot support any triangle like $\Delta_{uwv_r}$. For illustration see fig~\ref{fig:demand-two-doubly-attached-one-type-3-one-type-1}.
         
         \input{tikz_figures/demand-two-doubly-attached-one-type-3-one-type-1-common-type-3}

        %  *********OLD PROOF FOR COMMON TYPE-3*******

        %  Notice that the anchoring vertex for the attached triangles of $\psi^3$ must not be in $V(\psi \cup \psi_r)$ because $\psi_\ell$ shares an edge with all
        %  vertices in $V(\psi \cup \psi_r) \setminus V(\psi_\ell)$.
        %  And there are two ways (upto ) to draw $\psi^3$, (1) $\psi^3$ shares a vertex with $\psi_r$ and (2) $t_\ell$ does not share a vertex with $\psi_r$.

        %  In both the cases, there is an improving swap by substituting $\psi, \psi_r, \psi_\ell$ with $t_r, t_\ell, t_{rd}$ and an attached triangle of $\psi_\ell$. This follows from the key observation that none of $t_r, t_\ell, t_{rd}$ cannot share their edges among each other or a blue edge with any attached triangle of $\psi_\ell$ (since the anchoring vertex is not in $V(\psi \cup \psi_r)$.). Also, they together use exactly two green edges of $\psi_\ell$, hence we can pick the attached triangle of $\psi_\ell$ adjacent to the third edge ensuring that the new solution is a valid solution.

        %  % In the first case, there exists an improving swap by substituting $\psi, \psi_r, \psi_\ell$ with $t_r, t_\ell, t_{rd}$ and an attached triangle of $\psi_\ell$. In the second case, there exists a similar improving swap. The only different is only that we have to choose different attached triangle of $\psi_\ell$.

        %  \input{tikz_figures/demand-two-doubly-attached-one-type-3-one-type-1-common-t_rr}

        %  \input{tikz_figures/demand-two-doubly-attached-one-type-3-one-type-1-common-not-t_rr}

        %  *********OLD PROOF ENDS HERE*******
         
         \item \cat{$\psi_\ell$ and $\psi_r$ are type-$1$} In this case, we name the triangles $t_{rr}$ and $\psi_{rr}$ and their vertices as in the previous case. We also name $\psi_{\ell \ell}$ and $t_{\ell \ell}$ similarly (see fig~\ref{fig:demand-two-doubly-attached-two-type-1}). Note that $\psi_\ell$ and $\psi_r$ cannot be the same as $t\ell$ and $t_r$ need to be adjacent to the poor base edges of $\psi_\ell$ and $\psi_r$ respectively.
         If $\psi_{\ell \ell} \neq \psi_{rr}$, then in both cases when $v_\ell=v_r=v$ or when $u_\ell=u_r=u$ are impossible since there exists a solution improving $5$-swap by replacing the set of triangles $\sset=\{\psi, \psi_\ell, \psi_{\ell\ell}, \psi_r, \psi_{rr}\}$ by set $\sset'= \{t'_\ell, t_{\ell\ell}, t_\ell, t_r, t_{rr}, t'_r\}$, where $t'_\ell$ and $t'_r$ are the singly-attached triangles of $\psi_{\ell \ell}$ and $\psi_{rr}$ attached to edge $\overbar{w_{\ell \ell} x_{\ell\ell}}$ and  $\overbar{w_{rr} x_{rr}}$ respectively. It is easy to that the triangles in $\sset'$ are edge disjoint even in the worst case when $anchor(\psi_{\ell \ell}) = anchor(\psi_{rr})$. For illustration see fig~\ref{fig:demand-two-doubly-attached-two-type-1}).
         
        \input{tikz_figures/demand-two-doubly-attached-two-type-1}
            
         Otherwise $\psi_{\ell \ell} = \psi_{rr} =\psi^3$. Note that $\psi^3$ must contain the vertices $v_{\ell\ell}$ and $v_{rr}$ to make the edges $\overbar{v_\ell w_\ell}$ and $\overbar{v_r w_r}$ poor base edges for triangles $\psi_\ell$ and $\psi_r$ respectively. It should also contain $anchor(\psi_\ell)$ and $anchor(\psi_r)$. Let the third vertex of $\psi^3$ be $w$. 
         
         In case when $v_\ell = v_r = v$, the anchoring vertex for the singly attached triangles of $\psi_\ell$ and $\psi_r$ both has to be $w$, because $\overbar{v w_\ell}$ and $\overbar{v w_r}$ are suppose to be the poor base edges and $vv_{rr}$ and $vv_{\ell\ell}$ are already solution edges. This also implies that $w \notin \{v, u_\ell, u_r, w_\ell, w_r\}$. But this case is impossible since there exists a solution improving $4$-swap by replacing the set of triangles $\sset=\{\psi, \psi_\ell, \psi_r, \psi^3\}$ by set $\sset'= \{t_{\ell\ell}, t_\ell, t_r, t_{rr}, t'\}$, where $t'$ is the singly-attached triangles of $\psi^3$ attached to edge $\overbar{v_{\ell \ell} v_{rr}}$. It is easy to that the triangles in $\sset'$ are edge disjoint even in the worst case when $anchor(\psi^3)$ is common with one of the only possible vertices out of $\{u_\ell, u_r\}$. For illustration see fig~\ref{fig:demand-two-doubly-attached-two-type-1-common-type-3-v}.
         
        \input{tikz_figures/demand-two-doubly-attached-two-type-1-common-type-3-v}
            
         The only case left is when $u_\ell=u_r=u$ given that $\psi_{\ell \ell} = \psi_{rr} =\psi^3$. In this case the third vertex $w$ cannot be any of the already defined vertices in $\{v_\ell, v_r, w_\ell, w_r\}$ as $\psi^3$ should be edge disjoint from other solution triangles in $\{\psi, \psi_\ell, \psi_r\}$. In this case, both the anchoring vertex for the singly attached triangles of $\psi_\ell$ and $\psi_r$ cannot be $w$, otherwise the edge $\overbar{v_\ell w}$ and $\overbar{v_r w}$ will lead to an attachment for $\psi$ which is not possible as it is type-$0$. For illustration see fig~\ref{fig:demand-two-doubly-attached-two-type-1-common-type-3-attachment}.

        \input{tikz_figures/demand-two-doubly-attached-two-type-1-common-type-3-attachment}
            
         So either $anchor(\psi_\ell) = v_{rr}$ or $anchor(\psi_r) = v_{\ell\ell}$ (or both). 
         
         First let us argue for the case when one of the anchoring vertex is $w$. By renaming, we can assume $anchor(\psi_\ell) = w$, which implies $anchor(\psi_r) = v_{\ell\ell}$ and $w$ cannot be same as $u$. But this case is impossible since there exists a solution improving $4$-swap by replacing the set of triangles $\sset=\{\psi, \psi_\ell, \psi_r, \psi^3\}$ by set $\sset'= \{t_{\ell\ell}, t_\ell, t_r, t_{rr}, t'\}$, where $t'$ is the singly-attached triangles of $\psi^3$ attached to edge $\overbar{w v_{rr}}$. It is easy to that the triangles in $\sset'$ are edge disjoint. For illustration see fig~\ref{fig:demand-two-doubly-attached-two-type-1-common-type-3-anchor-w}.

        \input{tikz_figures/demand-two-doubly-attached-two-type-1-common-type-3-anchor-w}
            
        Finally the case left to argue is when $u_\ell=u_r=u$ given that $\psi_{\ell \ell} = \psi_{rr} =\psi^3$. Moreover, $anchor(\psi_\ell) = v_{rr}$ and $anchor(\psi_r) = v_{\ell\ell}$. This is the only case where $w$ could possibly be $u$. Note that this is a special case since $t_{\ell\ell}$ and $t_{rr}$ share a common edge $v_{\ell\ell} v_{rr}$, hence we cannot use them both for an improving swap. But still there exists another solution improving $4$-swap by replacing the set of triangles $\sset=\{\psi, \psi_\ell, \psi_r, \psi^3\}$ by set $\sset'= \{t_{\ell\ell}, t_\ell, t_r, t'_{rr}, t'\}$, where $t'$ is the singly-attached triangles of $\psi^3$ attached to edge $\overbar{w v_{rr}}$ and $t'_{rr} = \Delta_{v_{\ell\ell} v_\ell v_r}$. It is easy to that the triangles in $\sset'$ are edge disjoint even in the worst case when $w=u$. For illustration see fig~\ref{fig:demand-two-doubly-attached-two-type-1-common-type-3-anchors-vll-vrr}.

        \input{tikz_figures/demand-two-doubly-attached-two-type-1-common-type-3-anchors-vll-vrr}

        %  ***********************

        %  Otherwise $\psi^3_\ell = \psi^3_r$.
        %  Let $v_\ell$ be the vertex of $\psi^3_\ell$ that shares with $\psi_\ell$ and let $v_{r}$ be the vertex of $\psi^3_\ell$ that shares with $\psi_r$. \sumii{Notice that $v_{r} \neq v_\ell$, otherwise the structure cannot be realized.} Also let $v$ be the third vertex of $\psi^3_\ell$. For $t_{\ell d}$ ($t_{rd}$), the vertex that does not share with $\psi_\ell$ ($v_{rr}$) is either $v_{r}$ or $v$ ($v_{\ell}$ or $v$, respectively).
        %  If $v \in V( t_{\ell d} ) \cup V(t_{rd})$\sumii{, then two different green edges of $t_\ell3$ participate in $t_{\ell d}$ and $t_{rd}$.} Hence there exists an improving swap by substituting $\psi, \psi_\ell, \psi_r, \psi^3_\ell$ with $t_\ell, t_{r}, t_{\ell d}, t_{rd}$ and one attached triangle of $\psi^3_\ell$.

        %  Otherwise, we cannot choose $t_{\ell d}$ and $t_{rd}$ at the same time (see Fig.~\ref{fig:demand-two-doubly-attached-two-type-1-common-type-3-case3}). \sumii{Let $v'_\ell = V(t_{\ell \ell}) \cap V(\psi)$, $v''_\ell = V(t_{\ell \ell}) \setminus \{v_\ell, v'_\ell\}$ and similarly we define $v'_r, v''_r$. In this case, we can still have an improving swap by choosing doubly-attached triangles with vertices $\{v_\ell, v'_\ell, v'_r \}$ and $\{v''_\ell, v_\ell, v_r \}$, instead of $t_{\ell d}, t_{r d}$.}

      \end{enumerate}
   \end{proof}

    \begin{lemma}
      \label{lem:one-doubly-attached-demanding}
      If $t_\ell$ is doubly-attached, then $t_r$ cannot be hollow.
    \end{lemma}
    \begin{proof}
      Suppose not, then $t_\ell$ is doubly-attached triangle and $t_r$ a hollow triangle sharing demanding edges $e_\ell \neq e_r$ with $\psi$. There are three possible structures which involve the hollow triangle $t_r$
      (Fig~\ref{fig:hollow-0,3,3-demanding},\ref{fig:hollow-0,1,3-demanding}, ~\ref{fig:hollow-0,1,1-demanding}).
      Notice that in every case, there are two type-$3$ triangles involved.
      These type-$3$ triangles can be directly adjacent to $t_r$ or share a vertex with
      some type-$1$ triangle adjacent to $t_r$ such that it makes the base edge of the type-$1$ triangle poor which is also contained in $t_\ell$. Since there is exactly one type-$3$
      triangle involved in $t_\ell$ side's structure, hence there is at least one type-$3$ triangle
      of $t_r$ side, which does not share any edge with $t_\ell$ side.
      Let $\psi^3_r$ be such a type-$3$ triangle. There are two cases:
      \begin{enumerate}
         \item \cat{$\psi^3_r$ shares an edge with $t_r$} In this case, we
         substitute $\psi^3_r$ with its attached triangle. It is clear that
         if the initial packing solution is optimal, this substituted solution
         is also optimal. Moreover, $t_r$ is now doubly-attached which demands credits from $e_r$.
         
            \input{tikz_figures/demand-one-doubly-attached-one-hollow-type_r-adjacent-t_r3}

         \item \cat{$\psi^3_r$ does not share any edge with $t_r$} In this case, there exists a type-$1$ triangle $\psi_r$ which shares an edge with $t_r$ and share a vertex with $\psi^3_r$ and a doubly-attached triangle $t_{rr}$ which share one edge with $\psi_r$ and one edge with $\psi^3_r$. We substitute $\psi_r$ and $\psi^3_r$ by $t_{rr}$ and
         an attached triangle of $\psi^3_r$ to create an alternate optimal
         packing solution. As in previous case, $t_r$ is now doubly-attached which demands credits from $e_r$.

            \input{tikz_figures/demand-one-doubly-attached-one-hollow-type_r-adjacent-t_r1}

      \end{enumerate}
      In both case, we create scenarios where there both $t_\ell$ and $t_r$ are doubly-attached. Notice that both of them will still demanding credit from $\psi$, but this is impossible by
      Lemma~\ref{lem:both-doubly-attached-demanding}.
      Hence, this is a contradiction.
    \end{proof}

    \begin{lemma}
      If $t_\ell$ is hollow, then $t_r$ cannot be hollow.
    \end{lemma}
    \begin{proof}
      Suppose not, then $t_\ell$ and $t_r$ are hollow triangles sharing demanding edges $e_\ell \neq e_r$ with $\psi$. Now both $t_\ell$ side and $t_r$ side each have two type-$3$ triangles involved. If there exists a type-$3$ triangle which does not share any edge with the other side, then we can perform one of the non-improving swap, as used in the proof of
      Lemma~\ref{lem:one-doubly-attached-demanding}. Then this
      lead to a contradiction since by Lemma~\ref{lem:one-doubly-attached-demanding}, it is impossible to have a hollow triangle and a doubly-attached triangle both demanding credits from $\psi$.

      The same proof strategy holds even when there exists a type-$3$ triangle which shares an edge with one hollow triangle (also share a vertex with $\psi$). In this case, we argue that there is a non-improving swap that turns one hollow triangle into doubly-attached triangle without changing the picture of another hollow triangle. We then apply Lemma~\ref{lem:one-doubly-attached-demanding} as in the previous case.

      Suppose there is no such type-$3$ triangle, then the picture must be that both hollow triangles are of type-$[0,1,1]$. Moreover, there exists a type-$3$ triangle $\psi_3$ such that the doubly-attached triangles adjacent to $\psi_3$ drain credits from two type-$1$ triangle $\psi_{\ell}$ and $\psi_{r}$, one from each side.
      There exists an edge $e_1$ of $\psi_3$ such that if this edge becomes a non-solution edge, then $\psi_{\ell}$ will become type-$3$. Similarly, there exists an edge $e_2$ of $\psi_3$ such that if this edge turns blue, then $\psi_{r}$ will become type-$3$. We then perform a non-improving swap by substituting $\psi_3$ with one of its attached triangles. By choosing the base edge carefully (there exists $e^\prime \notin \{e_1, e_2\}$ of $\psi_3$), we can turn both $\psi_{\ell}$ and $\psi_{r}$ into   type-$3$ at the same time. Hence, we can again implement the strategy used in the previous cases to show a contradiction.

      % Suppose there is no such type-$3$ triangle, then there exists a type-$3$ triangle which substituting it with its attached triangle will turn some type-$1$ triangle(s) into type-$3$ triangles. Now we can apply the argument in the previous case above.

     Hence $t_r$ cannot be hollow.
    \end{proof}

    By three lemma above combined, $t$ cannot have two demanding edges.

    % Suppose the structures of two sides do not interact, then on each side, there exists a non-improving swap. When we perform the non-improving swaps of both side, then we get a better solution since they share only $\psi$.
    %
    % Now the difficult part. It is possible that the structures of two sides are interacted. We will list them below.
    %
    %
\end{proof}

\subsection{Proof of Lemma~\ref{lem:draining-doubly-attached}}

\begin{proof}
   Suppose the statement is false, then there are two cases.
   \begin{enumerate}
      \item \cat{$t$ has two drained edges} Let $\psi_{\ell}$ and $\psi_{r}$ be the type-$1$ triangles immediately next to $t$. Note that $\psi_{\ell} \neq \psi_{r}$ or they are not type-$1$.
      Similarly, let $t_{\ell}$ and $t_{r}$ be the doubly-attached triangles next to $\psi_{\ell}$ and $\psi_{r}$. We pick $t_\ell$ and $t_r$ in such a way that $V(t_\ell) \cap V(t_r) \cap V(t) = \varnothing$. Let $\psi_{\ell\ell}$ and $\psi_{rr}$ be the type-$3$ triangles next to $t_{\ell}$ and $t_{r}$. One can depict them from left-to-right as $\psi_{\ell\ell} t_{\ell} \psi_{\ell} t \psi_{r} t_{r} \psi_{rr}$.
      $\psi_{\ell\ell}$ can possibly be the same triangle as $\psi_{rr}$ (see Fig.~\ref{fig:type-[1,1]-two-drain-cycle}).
      In any case, by substituting $S=\{\psi_{\ell\ell}, \psi_{\ell}, \psi_{r}, \psi_{rr}\}$ with $S^\prime = \{t, t_{\ell}, t_{r}, t_1, t_2\}$ where $t_1$ and $t_2$ are the singly attached triangles which based on the edges $E(\psi_{\ell\ell}) \setminus E(t_\ell \cup t_r)$ and $E(\psi_{rr}) \setminus E(t_\ell \cup t_r)$, respectively.
      Since $|S^\prime| = |S| + 1$, we get a better packing solution.
      Hence this is a contradiction.
        \input{tikz_figures/type-1-1-two-drain}

    \input{tikz_figures/type-1-1-two-drain-cycle}
    %\sumi{Some polishing can be done here.}
      \item \cat{$t$ has one drained edge} but another green edge
      is not a non-drained base edge of some type-$1$ triangle.
      Let $\psi_{\ell}$ be the type-$1$ triangle which share drained edge with $t$ and let $\psi_r$ be the triangle which share another green edge with $t$. Note that $\psi_r$ is not type-$0$, hence $\psi_r$ has at least one base edge that is not shared with $t$.
      Also, let $t_{\ell}$ and $\psi_{\ell\ell}$ be defined similar to the previous case. Note that $\psi_r \neq \psi_{\ell\ell}$ or some edges cannot be realized. By substituting $S= \{ \psi_r, \psi_{\ell}, \psi_{\ell\ell}\}$ with
      $S^\prime = \{t, t_{\ell}, t_1, t_2\}$ where $t_1$ and $t_2$ are a singly-attached triangles of $\psi_{\ell\ell}$ and $\psi_{r}$, there exists a better solution. Note that $anchor(\psi_{\ell\ell})$ and $anchor(\psi_r)$ might be the same vertex, but even in that case, singly-attached triangles of $\psi_{\ell\ell}$ and singly-attached triangles of $\psi_r$ are pair-wise disjoint.
        \input{tikz_figures/type-1-3-one-drain}

        \input{tikz_figures/type-1-1-one-drain-one-non-base}
   \end{enumerate}
\end{proof}

\subsection{Proof of Lemma~\ref{lem:draining-hollow}}
\begin{proof}
   Suppose the statement above is not true, then there are four cases.
   \begin{enumerate}
      \item \cat{$t$ has three drained edges} In this case, there exists a side where the structure does not interact with other sides (e.g., $\Delta_{cde}$ side in Fig~\ref{fig:type-[1,1,1]-hollow-three-drain-common-type-3}). Otherwise, the type-$3$ triangle cannot be realized.
      By performing a non improving swap on that side (i.e., substituting $\Delta_{cde}$ and $\Delta_{exy}$ with $\Delta_{dex}$ and $\Delta_{jxy}$, an attached triangle attaching to $\Delta_{exy}$ in Fig~\ref{fig:type-[1,1,1]-hollow-three-drain-common-type-3}), without decrease the number of triangles in our packing solution, we create a situation where $t$ becomes a doubly-attached triangle with two drained edges. Recall that Lemma~\ref{lem:draining-doubly-attached} says that any doubly-attached triangle can have at most one drained edge. Hence, this is impossible.
    \input{tikz_figures/type-1-1-1-hollow-three-drain}
    \input{tikz_figures/type-1-1-1-hollow-three-drain-common-type-3}
    %%%%%%%%%%
    \item \cat{$t$ has two drained edges} but the third edge is not a non-drained base edge of some type-$1$ triangle. Then it is either a non-drained non-base edge of a type-$1$ triangle  or an edge of type-$3$ triangle. As in previous case, by performing a non-improving swap by substituting the type-$1$/type-$3$ triangle by its supported triangle which is not adjacent to $t$, we again create the situation where $t$ becomes a doubly-attached triangle with two drained edges, that is impossible by Lemma~\ref{lem:draining-doubly-attached}.  Hence this is a contradiction.
    \input{tikz_figures/type-1-1-1-hollow-two-drain-non-base}
    \input{tikz_figures/type-1-1-1-hollow-two-drain-non-base-common-type-3}
    \input{tikz_figures/type-1-1-3-hollow-two-drain}
    \input{tikz_figures/type-1-1-3-hollow-two-drain-common-type-3}
    %%%%%%%%%%
      \item \cat{$t$ has one drained edge and $t$ is adjacent to two type-$3$ triangles} We can perform a non-improving swap, substituting a type-$3$ triangle adjacent to $t$ with its attached triangle, to create the situation in which $t$ is a doubly attached triangle with one drained edge and other edge from a type-$3$ triangle, that is impossible by Lemma~\ref{lem:draining-doubly-attached}. Hence this is a contradiction.

    \input{tikz_figures/type-1-3-3-hollow-one-drain}

      \item \cat{$t$ has one drained edge, one non-drained non-base edge from type-$1$ triangle, and one edge from type-$3$ triangle} As in the previous case, we can perform a non-improving swap by substituting the type-$3$ triangle with its attached triangle. Since the result structure violates Lemma~\ref{lem:draining-doubly-attached}, this is a contradiction.
    %\begin{figure}[H]
    %    \centering
    %    \includegraphics[width=0.6\textwidth]{figures/type-[1,1,1]-hollow-one-drain-two-non-base.png}
    %    \caption{One drain edges for type-$[1, 1, 1]$ hollow triangle with two non-base edges of type-$1$ triangles}
    %    \label{fig:type-[1,1,1]-hollow-one-drain-two-non-base}
    %\end{figure}

    \input{tikz_figures/type-1-1-3-hollow-one-drain-one-non-base}

   \end{enumerate}
   As all the cases lead to contradiction, the only remaining cases are the ones stated in the lemma. This completes the proof.
\end{proof}

% Since we exhaust all the cases, there cannot be any other structure.

\section{Relations between multi-transversals of various orders}
\label{app:relation-btw-multi-transversals}
In this section, we explain why  $\tau^*_2(G)$ or $\tau^*_3(G)$ are not subsumed by each other.

\begin{claim}
There is an infinite family of graphs $G$ for which $\tau^*_2(G) \leq (\frac{3}{4}+o(1)) \tau^*_3(G)$
\end{claim}
\begin{proof}
We will illustrate a family of $n$-vertex graphs $G_n$ where $\tau^*_2(G_n) = \frac{n}{2}$ but $\tau^*_3(G_n) = \frac{2}{3}(1-o(1)) n$.
By~\cite{kortsarz2010approximating}, it suffices to construct a triangle-free graph $G_n$ where the gap exists between the fractional and integral optimal solutions of the vertex cover problem.
We consider a triangle-free graph $G_n$ where ${\sf VC}(G_n) = (1-o(1))n$ (this is just a random graph $G(n,p)$ with appropriate parameter and using the alteration steps to remove all triangles). 
In any graph, there is a fractional feasible cover of value $n/2$ (by assigning $1/2$ everywhere), so we have that $\tau^*_2(G) \leq n/2$. 

Now we analyze $\tau^*_3(G)$. Consider any $\frac{1}{3}$-integral assignment $z$ on vertices $V(G_n)$. Partition $V(G_n)$ based on the assigned $z$-values into $V_0, V_{1/3}$, $V_{2/3}$, and $V_{1}$.
Notice that $V_0 \cup V_{1/3}$ must be an independent set, for otherwise an edge $e \in G[V_0 \cup V_{1/3}]$ would violate the covering constraint. 
Therefore, $|V_0 \cup V_{1/3}| = o(n)$ (since the size of any independent set in $G$ is at most $o(n)$).
This implies that the total assignment must be at least $\frac{2}{3} (1-o(1)) n$.
\end{proof}

\begin{claim}
There is an infinite family of graphs $G$ for which $\tau^*_3(G) \leq \frac{5}{6} \tau^*_2(G)$.
\end{claim}
\begin{proof}
We show that this gap holds in the case of a complete graph on $6$ vertices.
In particular, $\tau^*_3(K_6) \leq 5$ but $\tau^*_2(K_6) \geq 6$.
The first claim is easy, since we can simply assign $1/3$ on each edge, and there are $15$ edges in the graph. 
The second claim relies on Proposition~\ref{prop: complete graphs} to say that $\tau^*_2(K_6)\geq 6$. 
\end{proof}
