# Supplementary material for: Multi-transversals for Triangles and the Tuza's Conjecture
Source: arXiv:2001.00257 source file (2021-02-03)
Supplement: Supplementary file 3 [file appendix2.33.tex]

\section{Missing proof for Section~\ref{sec:type-13-transversal}}
